# Supplementary material for: Do Large Multimodal Models Solve Caption Generation for Scientific Figures? Lessons Learned from SciCap Challenge 2023
Source: arXiv:2501.19353 source file (2025-02-18)
Supplement: Supplementary file 1 [file Appendix.tex]

\label{sec:appendix}
\newpage

\section{Additional Experimental Results}
\begin{table*}[ht!]
\centering

\scalebox{0.8}{
\begin{tabular}{lccccccccc}
\hline
\multirow{2}{*}{\textbf{Model}} & \multirow{2}{*}{\textbf{Domain}} & \multirow{2}{*}{\textbf{Token Length}} & \multirow{2}{*}{\textbf{BLEU-4}} & \multicolumn{2}{c}{\textbf{Rouge-1}} & \multicolumn{2}{c}{\textbf{Rouge-2}} & \multicolumn{2}{c}{\textbf{Rouge-L}} \\  
 \cmidrule(lr){5-10}
         &    &  & & \textbf{Score} & \textbf{Norm} & \textbf{Score} & \textbf{Norm} & \textbf{Score} & \textbf{Norm}\\
\hline
GPT-4V (img) & physics & 20.7 & .003 & .167 & 0.900 & .039 & 0.640 & .131 & 0.863 \\
 & cs & 17.5 & .004 & .198 & 1.096 & .053 & 0.900 & .163 & 1.096 \\
 & math & 17.6 & .002 & .146 & 0.821 & .027 & 0.480 & .121 & 0.826 \\
 & q-bio & 18.2 & .004 & .171 & 0.959 & .045 & 0.783 & .137 & 0.930 \\
 & stat & 17.5 & .003 & .190 & 1.060 & .046 & 0.790 & .151 & 1.024 \\
 & q-fin & 18.0 & .002 & .146 & 0.857 & .033 & 0.607 & .116 & 0.818 \\
 & eess & 18.1 & .004 & .212 & 1.160 & .056 & 0.942 & .173 & 1.154 \\
 & econ & 18.8 & .004 & .172 & 0.965 & .051 & 0.894 & .146 & 0.991 \\
\hline

Pegasus inlg para+ocr-caption-30 & physics & 32.6 & .049 & .243 & 1.237 & .120 & 1.846 & .202 & 1.283 \\
 & cs & 19.5 & .162 & .379 & 2.218 & .270 & 4.958 & .357 & 2.504 \\
 & math & 20.6 & .092 & .276 & 1.689 & .177 & 3.441 & .257 & 1.866 \\
 & q-bio & 31.4 & .078 & .278 & 1.407 & .155 & 2.369 & .239 & 1.508 \\
 & stat & 25.8 & .128 & .332 & 1.770 & .222 & 3.619 & .305 & 1.997 \\
 & q-fin & 24.6 & .066 & .281 & 1.525 & .163 & 2.720 & .250 & 1.656 \\
 & eess & 18.1 & .182 & .410 & 2.509 & .298 & 5.813 & .388 & 2.825 \\
 & econ & 25.6 & .092 & .315 & 1.661 & .207 & 3.328 & .297 & 1.929 \\
\hline
Pegasus inlg para-caption-6 & physics & 20.8 & .042 & .239 & 1.415 & .126 & 2.355 & .208 & 1.470 \\
 & cs & 12.5 & .082 & .330 & 2.358 & .198 & 4.731 & .307 & 2.530 \\
 & math & 14.2 & .061 & .263 & 1.959 & .153 & 3.870 & .243 & 2.076 \\
 & q-bio & 19.3 & .051 & .265 & 1.587 & .143 & 2.702 & .233 & 1.668 \\
 & stat & 15.8 & .069 & .290 & 1.880 & .166 & 3.488 & .263 & 2.007 \\
 & q-fin & 15.4 & .046 & .268 & 1.751 & .153 & 3.236 & .240 & 1.841 \\
 & eess & 12.0 & .102 & .365 & 2.655 & .228 & 5.572 & .339 & 2.849 \\
 & econ & 16.8 & .064 & .297 & 1.874 & .175 & 3.542 & .272 & 2.022 \\
\hline
\end{tabular}
}
\caption{Results breakdown by domain for each model, highlighting performance metrics such as BLEU-4, Rouge scores, and token length.}
\label{tab:appendix_results_by_domain}
\end{table*}

\begin{table*}[ht!]
\centering

\resizebox{\linewidth}{!}{
\begin{tabular}{lccccccccc}
\hline
\multirow{2}{*}{\textbf{Model}} & \multirow{2}{*}{\textbf{Type}} & \multirow{2}{*}{\textbf{Token Length}} & \multirow{2}{*}{\textbf{BLEU-4}} & \multicolumn{2}{c}{\textbf{Rouge-1}} & \multicolumn{2}{c}{\textbf{Rouge-2}} & \multicolumn{2}{c}{\textbf{Rouge-L}} \\  
 \cmidrule(lr){5-10}
         &    &  & & \textbf{Score} & \textbf{Norm} & \textbf{Score} & \textbf{Norm} & \textbf{Score} & \textbf{Norm}\\
\hline
GPT-4V (img) & Node Diagram & 16.7 & .001 & .163 & 0.897 & .032 & 0.548 & .135 & 0.907 \\
 & Equation & 18.0 & .001 & .142 & 0.762 & .025 & 0.410 & .118 & 0.772 \\
 & Graph Plot & 19.9 & .004 & .187 & 1.014 & .048 & 0.809 & .148 & 0.985 \\
 & Scatterplot & 20.8 & .003 & .169 & 0.904 & .040 & 0.647 & .131 & 0.859 \\
 & Bar Chart & 16.6 & .004 & .203 & 1.187 & .057 & 1.045 & .170 & 1.192 \\
\hline
Pegasus inlg para+ocr-caption-30 & Node Diagram & 18.9 & .084 & .294 & 1.689 & .173 & 3.114 & .271 & 1.876 \\
 & Equation & 21.8 & .069 & .263 & 1.468 & .146 & 2.516 & .236 & 1.594 \\
 & Graph Plot & 28.6 & .119 & .321 & 1.705 & .211 & 3.433 & .289 & 1.886 \\
 & Scatterplot & 31.3 & .049 & .248 & 1.263 & .120 & 1.853 & .207 & 1.311 \\
 & Bar Chart & 21.2 & .069 & .291 & 1.647 & .152 & 2.680 & .257 & 1.756 \\
\hline
Pegasus inlg para-caption-6 & Node Diagram & 11.6 & .081 & .308 & 2.281 & .183 & 4.586 & .288 & 2.454 \\
 & Equation & 14.0 & .061 & .273 & 1.864 & .153 & 3.441 & .250 & 1.991 \\
 & Graph Plot & 18.4 & .058 & .277 & 1.721 & .158 & 3.152 & .247 & 1.822 \\
 & Scatterplot & 19.5 & .041 & .237 & 1.427 & .122 & 2.338 & .206 & 1.480 \\
 & Bar Chart & 13.9 & .064 & .313 & 2.108 & .169 & 3.731 & .283 & 2.228 \\
\hline
\end{tabular}
}
\caption{Results breakdown by type for each model, highlighting performance metrics such as BLEU-4, Rouge scores, and token length.}
\label{tab:appendix_results_by_type}
\end{table*}
