# Supplementary material for: Do Large Multimodal Models Solve Caption Generation for Scientific Figures? Lessons Learned from SciCap Challenge 2023
Source: arXiv:2501.19353 source file (2025-02-18)
Supplement: Supplementary file 3 [file appendix_results_figuretype.tex]

\begin{table*}[ht!]
\centering

\resizebox{\linewidth}{!}{
\begin{tabular}{lccccccccc}
\hline
\multirow{2}{*}{\textbf{Model}} & \multirow{2}{*}{\textbf{Type}} & \multirow{2}{*}{\textbf{Token Length}} & \multirow{2}{*}{\textbf{BLEU-4}} & \multicolumn{2}{c}{\textbf{Rouge-1}} & \multicolumn{2}{c}{\textbf{Rouge-2}} & \multicolumn{2}{c}{\textbf{Rouge-L}} \\  
 \cmidrule(lr){5-10}
         &    &  & & \textbf{Score} & \textbf{Norm} & \textbf{Score} & \textbf{Norm} & \textbf{Score} & \textbf{Norm}\\
\hline
GPT-4V (img) & Node Diagram & 16.7 & .001 & .163 & 0.897 & .032 & 0.548 & .135 & 0.907 \\
 & Equation & 18.0 & .001 & .142 & 0.762 & .025 & 0.410 & .118 & 0.772 \\
 & Graph Plot & 19.9 & .004 & .187 & 1.014 & .048 & 0.809 & .148 & 0.985 \\
 & Scatterplot & 20.8 & .003 & .169 & 0.904 & .040 & 0.647 & .131 & 0.859 \\
 & Bar Chart & 16.6 & .004 & .203 & 1.187 & .057 & 1.045 & .170 & 1.192 \\
\hline
Pegasus inlg para+ocr-caption-30 & Node Diagram & 18.9 & .084 & .294 & 1.689 & .173 & 3.114 & .271 & 1.876 \\
 & Equation & 21.8 & .069 & .263 & 1.468 & .146 & 2.516 & .236 & 1.594 \\
 & Graph Plot & 28.6 & .119 & .321 & 1.705 & .211 & 3.433 & .289 & 1.886 \\
 & Scatterplot & 31.3 & .049 & .248 & 1.263 & .120 & 1.853 & .207 & 1.311 \\
 & Bar Chart & 21.2 & .069 & .291 & 1.647 & .152 & 2.680 & .257 & 1.756 \\
\hline
Pegasus inlg para-caption-6 & Node Diagram & 11.6 & .081 & .308 & 2.281 & .183 & 4.586 & .288 & 2.454 \\
 & Equation & 14.0 & .061 & .273 & 1.864 & .153 & 3.441 & .250 & 1.991 \\
 & Graph Plot & 18.4 & .058 & .277 & 1.721 & .158 & 3.152 & .247 & 1.822 \\
 & Scatterplot & 19.5 & .041 & .237 & 1.427 & .122 & 2.338 & .206 & 1.480 \\
 & Bar Chart & 13.9 & .064 & .313 & 2.108 & .169 & 3.731 & .283 & 2.228 \\
\hline
\end{tabular}
}
\caption{Results breakdown by type for each model, highlighting performance metrics such as BLEU-4, Rouge scores, and token length.}
\label{tab:appendix_results_by_type}
\end{table*}
